# Supplementary material for: Flexible Control Flow Graph Alignment for Delivering Data-Driven Feedback to Novice Programming Learners
Source: arXiv:2401.01416 source file (2024-01-02)
Supplement: Supplementary file 1 [file appendix.tex]

\section{Qualitative Analysis}

\begin{figure}
\centering
\includegraphics[scale=0.23]{successful_repair_by_problem.pdf}
\caption{Percentage of programs fully repaired grouped by programming problem}
\label{fig:successful_repair_by_problem}
\end{figure}

Our FA suggested the following changes:
\begin{enumerate}
    \item Change \pyth{for i in range(1,(n+1))} at line 2 to \pyth{for i in range(n)}
    \item Change \pyth{i%2!=0} to \pyth{i%2==0} at line 3
    \item Add \pyth{j = i//2} at line 8
    \item Change \pyth{print(srt)} at line 15 to \pyth{print("."+((m-1)*"."))}
    \item Change \pyth{print(srt)} at line 23 to \pyth{print("#"+((m-1)*"."))}
    \item Delete the assignments to \pyth{srt} at lines 4,9,12,14,17,20,22.
\end{enumerate}

% Correct
\newsavebox{\FAComparisonCorrect}
\begin{lrbox}{\FAComparisonCorrect}
\begin{minipage}[b]{0.4\textwidth}
\begin{python}
ip = input()
ipArr = ip.split(" ")
opp = False
height = int(ipArr[0])
width = int(ipArr[1])
for i in range(height):
  if (i + 1) % 2 == 0:
    if opp == False:
      for n in range(width - 1):
        print('.', end='')
      print('#')
      opp = True
  [truncated...]
  else:
    for j in range(width - 1):
      print('#', end='')
    print('#')
\end{python}
\end{minipage}
\end{lrbox}
% incorrect
\newsavebox{\FAComparisonInorrect}
\begin{lrbox}{\FAComparisonInorrect}
\begin{minipage}[b]{0.4\textwidth}
\begin{python}
def Snake(m,n):
  alternate=1                  
  for i in range(1,m+1):
    if alternate==1 and i%2==0:
      alternate=0
    elif alternate==0 and i%2==0:alternate=1    
      for j in range(1,n+1):
        [truncated...]
        else:print('#',end=" ")
    print("")    
m,n=map(int,input().split())
Snake(m,n)
\end{python}
\end{minipage}
\end{lrbox}
In the case of problem \textit{1360B}, $FA(L)$ outperforms $FA(L+E)$ i.e. using only semantic information performs better than using both semantic and topological information. The primary reason for that is our experimental consideration of halting comparison if the similarity score between the two programs fell below 0.6 as discussed in Section~\ref{subsec:exp_setup}. Considering both semantic and topological information results in the similarity score falling below 0.6 for a more significant portion of the problems in \textit{1360B} than simply considering semantic information.
Figure~\ref{fig:corr&inCorrForGMScore} displays the sample correct and incorrect programs for which $FA(L)$ results in a similarity score of 0.68, while $FA(L+E)$ results in a similarity score of 0.58. In this sample case, running through Algorithm~\ref{alg:GM} and taking into account edge similarity results in the similarity score falling below the threshold. Taking into account both semantic and topological should in theory decrease the similarity score between programs and we can see this in practice in this scenario.

\subsection{Threats to Validity}
% Correct
% \newsavebox{\gptcorrect}
% \begin{lrbox}{\gptcorrect}
% \begin{minipage}[b]{0.5\textwidth}
% \begin{python}
% n,m=map(int,input().split())
% for i in range(n):
%   print(['#'*m,'.'*(m-1)+'#','#'*m,'#'+'.'*(m-1)][i%4])
% \end{python}
% \end{minipage}
% \end{lrbox}
% % incorrect
% \newsavebox{\gptincorrect}
% \begin{lrbox}{\gptincorrect}
% \begin{minipage}[b]{0.5\textwidth}
% \begin{python}
% n,m=input().split()
% n=int(n)
% m=int(m)
% s=['#'*m,'*'*(m-1)+'#','#'*m,'#'+'*'*(m-1)]
% for i in range(n):
%  print(s[i%4])
% \end{python}
% \end{minipage}
% \end{lrbox}
% \begin{figure}[t]

% \centering
% \subfloat[Correct Program\label{fig:gptcorrect}]{\usebox{\gptcorrect}}~\quad\quad
% \subfloat[Incorrect Program\label{fig:gptincorrect}]{\usebox{\gptincorrect}}
% \caption{Correct and incorrect programs provided to ChatGPT}
% \label{fig:corr&inCorrChatGPT}
% \end{figure}

\subsection{Qualitative analysis}
\label{subsec:qual}

% % Correct
% \newsavebox{\GMStructMismatchCorrect}
% \begin{lrbox}{\GMStructMismatchCorrect}
% \begin{minipage}[b]{0.4\textwidth}
% \begin{python}
% n, m=map(int,input().split())
% for i in range(n):
%   if i % 2 == 0:
%     print("#"*m)
%   else:
%     a = i//2
%     if a % 2 == 0:
%       print("."*(m-1)+"#")
%     else:
%       print("#"+(m-1)*".")
% \end{python}
% \end{minipage}
% \end{lrbox}
% \newsavebox{\GMStructMismatchIncorrect}
% \begin{lrbox}{\GMStructMismatchIncorrect}
% \begin{minipage}[b]{0.4\textwidth}
% \begin{python}
% n, m=map(int,input().split())
% for i in range(1,n+1):
%   if i % 2 != 0:
%     srt = ''
%     for j in range(m):
%       srt += '#'
%       print(srt)
%   elif i % 4 == 2:
%     srt = ''
%     for i in range(m):
% [truncated ...] 
%   else:
%     srt = ''
%     for i in range(m):
% [truncated...]
% \end{python}
% \end{minipage}
% \end{lrbox}

% \begin{figure}
% \centering
% \subfloat[Correct program\label{fig:GMStructMismatchCorrect}]{\usebox{\GMStructMismatchCorrect}}~\quad\quad
% \subfloat[Incorrect program\label{fig:GMStructMismatchIncorrect}]{\usebox{\GMStructMismatchIncorrect}}
% \caption{Correct and incorrect programs used to illustrate control flow conflicts}
% \label{fig:corr&inCorrForStructMismatch}
% \end{figure}

For our qualitative analysis, we focus on Problem \textit{510A}, where FA achieves more than 50\% success rate while baseline CLARA fails completely. Furthermore,  $FA(L+E)$ significantly outperforms $FA(L)$ for programs in this problem; thus giving us two examples of the performance benefits of FA.

%\paragraph{Control flow conflicts} 
From a sample of 7 correct and 78 incorrect programs that comprise this problem. Figure~\ref{fig:corr&inCorrForFAComparison} presents an example of a comparison (correct and incorrect programs) that emphasizes the high degree of difference and dissociated control flows between the two programs. As can be seen, the correct program contains a single loop with two $\kw{if}$ statements embedded, while the incorrect program contains several nested loops and $\kw{if}$ statements. CLARA requires programs to have similar control flows in order to proceed with the repair process. Our flexible alignment does not have such a prerequisite and completes the repair process on these two programs, suggesting 12 repairs are required with a change percentage of 23\% and 24\% for this particular comparison.

% Correct
\newsavebox{\FAComparisonCorrect}
\begin{lrbox}{\FAComparisonCorrect}
\begin{minipage}[b]{0.4\textwidth}
\begin{python}
ip = input()
ipArr = ip.split(" ")
opp = False
height = int(ipArr[0])
width = int(ipArr[1])
for i in range(height):
  if (i + 1) % 2 == 0:
    if opp == False:
      for n in range(width - 1):
        print('.', end='')
[truncated...]
\end{python}
\end{minipage}
\end{lrbox}
% incorrect
\newsavebox{\FAComparisonInorrect}
\begin{lrbox}{\FAComparisonInorrect}
\begin{minipage}[b]{0.4\textwidth}
\begin{python}
def Snake(m,n):
  alternate=1                  
  for i in range(1,m+1):
    if alternate==1 and i%2==0:
      alternate=0
    elif alternate==0 and i%2==0:alternate=1    
      for j in range(1,n+1):
[truncated...] 
\end{python}
\end{minipage}
\end{lrbox}

\begin{figure}[h]
\centering
\subfloat[Correct Program\label{fig:GMScoreCorrect}]{\usebox{\FAComparisonCorrect}}~\quad\quad
\subfloat[Incorrect Program\label{fig:GMScoreIncorrect}]{\usebox{\FAComparisonInorrect}}
\caption{Sample programs where FA(L+E) succeeds but FA(L) fails. FA(L) fails to create the best model with only semantic information in our permutation limit of 1000.}
\label{fig:corr&inCorrForFAComparison}
\end{figure}

%\paragraph{Semantic vs.~topological information}
The sample code in Figure~\ref{fig:corr&inCorrForFAComparison} resulted in a similarity score of 0.75 for $FA(L)$ and 0.74 for $FA(L+E)$. 
However, the $FA(L)$ failed to find the best model whereas $FA(L+E)$ recommended a repair with a high percentage change (70\%) indicating that in cases where significant change is required between similarly modeled incorrect and correct programs - topological information is required to identify the best model.
